# Supplementary material for: Context-Based Tweet Engagement Prediction
Source: arXiv:2310.03147 source file (2023-09-28)
Supplement: Supplementary file 1 [file 1dFollows.tex]

\begin{lstlisting}[language=Python,caption={Code create the graph representing the first-degree following relations}, label=lst1dFollows]
import pyspark.sql.functions as f
from Functions.pyspark_df_shape import pyspark_df_shape


def extract_follows(df, flag_column=None, repartition=None, print_inter_counts=False):
    """
    Creates a comprehensive df with follows relations of the form <following_id, followed_id, flag_column> containing
    rows where <flag_column> indicates whether <following_id> follows <followed_id>.

    Parameters
    ----------
    df: Pyspark dataframe from which the graphs are built
    flag_column: if None, the graph will be of the form <following_id, followed_id> for the pairs with a follows
        relation; if it is a sting, then it will be of the form <following_id, followed_id, flag_column> with
        flag_column indicating whether following_id follows followed_id.
    repartition: if an int, will be reparitioned to the given number of columns first.
    print_inter_counts: whether to print counts of intermediary steps

    Returns a graph in PySpark dataframe of the form <following_id, followed_id> or
        <following_id, followed_id, flag_column>
    -------

    """
    
    if (repartition is not None) and (type(repartition) == int):
        df = df.repartition(repartition, 'engaging_user_id')

    # when following_id == engaging_user_id and followed_id == engaged_with_user_id, then 
    # the row will have <follows> = True by design of the dataset
    engaging_follows_engaged = df.select(['engaging_user_id', 'engaged_with_user_id']).distinct()
    engaging_follows_engaged = engaging_follows_engaged.withColumnRenamed('engaging_user_id', 'following_id')
    engaging_follows_engaged = engaging_follows_engaged.withColumnRenamed('engaged_with_user_id', 'followed_id')

    # add engaged users that explicitly follow engaging users
    engaged_follows_engaging = df.filter(f.col('engagee_follows_engager') == True) \
        .select(['engaged_with_user_id', 'engaging_user_id']).distinct()
    engaged_follows_engaging = engaged_follows_engaging.withColumnRenamed('engaged_with_user_id', 'following_id')
    engaged_follows_engaging = engaged_follows_engaging.withColumnRenamed('engaging_user_id', 'followed_id')

    # merge the previous two
    follows = engaging_follows_engaged.union(engaged_follows_engaging).distinct()
    
    if print_inter_counts:
        print("shape(follows) = ", pyspark_df_shape(follows, tpl = False))

    # if explicit flag_column is not required, just return a df with columns <following_id, followed_id>
    if flag_column is None:
        return follows

    # add those relations f or which we are sure that they do not follow each other
    negatives = df.filter(f.col('engagee_follows_engager') == False).select(
        ['engaged_with_user_id', 'engaging_user_id']).distinct()
    negatives = negatives.withColumnRenamed('engaged_with_user_id', 'following_id')
    negatives = negatives.withColumnRenamed('engaging_user_id', 'followed_id')

    if print_inter_counts:
        print("shape(negatives pre join) = ", pyspark_df_shape(negatives, tpl = False))
    
    # remove those which are actually true due to the first condition (there are indeed such cases, cf. http://prntscr.com/1v6j2bq)
    negatives = negatives.join(follows, on = ["following_id", "followed_id"], how='left_anti')
    
    if print_inter_counts:
        print("shape(negatives post join) = ", pyspark_df_shape(negatives, tpl = False))

    # set the <follows> flag
    follows = follows.withColumn(flag_column, f.lit(True))
    negatives = negatives.withColumn(flag_column, f.lit(False))

    # return the resulting graph <following_id, followed_id, flag_column>
    return follows.union(negatives)

\end{lstlisting}
