# Supplementary material for: Context-Based Tweet Engagement Prediction
Source: arXiv:2310.03147 source file (2023-09-28)
Supplement: Supplementary file 2 [file 2dFollows.tex]

\begin{lstlisting}[language=Python,caption={Code create the graph representing the second-degree following relations}, label=lst2dFollows]
import pyspark.sql.functions as f
from Functions.pyspark_df_shape import pyspark_df_shape


def extract_follows_2d(follows, flag_column=None, repartition=None, print_inter_counts=False):
    """
    Takes a follows graph of the first-degree connection of the form <following_id, followed_id> or
    <following_id, followed_id, flag_column> (cf. fe02_extract_follows.py) and creates a df of second-degree connections

    Parameters
    ----------
    follows: a first-degree follows graph, as created by function extract_follows
    flag_column: if None, the graph will be of the form <following_id, followed_id> for the pairs with a 2nd-degree
        follows relation; if it is a sting, then it will be of the form <following_id, followed_id, flag_column> with
        flag_column indicating whether following_id follows someone who follows followed_id.

    Returns a graph in PySpark dataframe of the form <following_id, followed_id> or
        <following_id, followed_id, flag_column>
    -------
    """
    
    if (repartition is not None) and (type(repartition) == int):
        follows = follows.repartition(repartition, 'engaging_user_id')

    left = follows.withColumnRenamed("following_id", "left_following_id").withColumnRenamed("followed_id", "left_followed_id")
    right = follows.withColumnRenamed("following_id", "right_following_id").withColumnRenamed("followed_id", "right_followed_id")

    if flag_column is not None:
        left = left.withColumnRenamed(flag_column, "left_" + flag_column)
        right = right.withColumnRenamed(flag_column, "right_" + flag_column)

    # join on the second (inner) user
    second_degree = left.join(right, left["left_followed_id"] == right["right_following_id"], how="inner")
    second_degree = second_degree.drop("left_followed_id").drop("right_following_id") \
        .withColumnRenamed("left_following_id", "following_id").withColumnRenamed("right_followed_id", "followed_id")

    if print_inter_counts:
        print("shape(second_degree after join) = ", pyspark_df_shape(second_degree, tpl = False))
    
    if flag_column is not None:
        # complicated case, check what the value of the flag should be:
        second_degree = second_degree.withColumn("temp_" + flag_column,
                                                 f.when(f.col("left_" + flag_column) & f.col("right_" + flag_column),
                                                        True).otherwise(False))
        second_degree = second_degree.drop("left_" + flag_column).drop("right_" + flag_column)
        # account for the fact that there may be multiple second degree connections between any two users, the max will
        # result in True if at least one of the rows is true; http://prntscr.com/1vkd1vf
        second_degree = second_degree.groupBy("following_id", "followed_id").agg(
            f.max("temp_" + flag_column).alias(flag_column))
        
        if print_inter_counts:
            print("shape(second_degree after groupBy) = ", pyspark_df_shape(second_degree, tpl = False))

    return second_degree.distinct()

\end{lstlisting}
