# Supplementary material for: Context-Based Tweet Engagement Prediction
Source: arXiv:2310.03147 source file (2023-09-28)
Supplement: Supplementary file 3 [file chiSqSelector.tex]

\begin{lstlisting}[language=Python, caption={Code that attepts to load pre-existing chi-squared selectors models if so desired and if they exist or that fits new chi-square selectors otherwise}, label=lstChiSqSelecor]
selector_models = {}
selected_features = {}

for key in vec_dfs:
    selector_models[key] = {}
    selected_features[key] = {}
    print(f"Now at {datetime.now().strftime('%d.%m.%Y %H:%M:%S')}, loading or recreating selectors for {key}.")
    for fs in featuresets:
        if "unscaled" in fs:
            print(f"\tSkipping chiSq selection for {key}/{fs} because chiSq requires binning.")
            continue
        selector_models[key][fs] = {}
        selected_features[key][fs] = {}
        for target in target_features:
            selector_models[key][fs][target] = {}
            selected_features[key][fs][target] = {}
            for number_of_top_features in [5, 10, 25, 50]:
                selector_does_not_exist = False

                if fs == "relevant_features":
                    selector_name = "chiSqSelector_"+str(number_of_top_features)+"_features_targeting_"+target+"_for_"+key
                else:
                    selector_name = "chiSqSelector_"+str(number_of_top_features)+"_"+fs+"_features_targeting_"+target+"_for_"+key
                selector_path = os.path.join(SELECTOR_FOLDER, selector_name)
                
                if not REWRITE_EXISTING_MODELS:
                    try:
                        selector_model = mlf.ChiSqSelectorModel.load(selector_path)
                        if CALCULATE_STEPS:
                            print(f"\tChiSqSelector for {target} with {number_of_top_features} {fs} features loaded from file.")
                    except (Py4JJavaError, FileNotFoundError, AnalysisException) as error:
                        selector_does_not_exist = True
                        changed_dfs.add(key)

                if REWRITE_EXISTING_MODELS or selector_does_not_exist:
                    if CALCULATE_STEPS:
                        print(f"\tChiSqSelector for {target} with {number_of_top_features} {fs} features must be recreated.")
                        
                    output_col = "selected_features_"+target if fs == "relevant_features" else "selected_"+fs+"_"+target
                    selector = mlf.ChiSqSelector(numTopFeatures=number_of_top_features,featuresCol=fs, fpr=0.05, 
                                                 outputCol=output_col, labelCol= target) 
                    selector_model = selector.fit(vec_dfs[key])
                    selector_model.write().overwrite().save(selector_path)

                selector_models[key][fs][target]["top_"+str(number_of_top_features)] = selector_model 
                selected_features[key][fs][target]["top_"+str(number_of_top_features)] = \
                                    [metadata_ordering[key][fs][i] for i in selector_model.selectedFeatures]
\end{lstlisting}
