# Supplementary material for: Context-Based Tweet Engagement Prediction
Source: arXiv:2310.03147 source file (2023-09-28)
Supplement: Supplementary file 4 [file evaluateAll.tex]

\begin{lstlisting}[language=Python, caption={The method used to fit and evaluate all forwarded combinations of source datasets, target datasets, and sets of features}, label={lstEvaluateAll}]
def mllib_evaluate_all(dfs,
                       target_features=('like', 'reply', 'retweet', 'quote', 'react'),
                       algorithm_name_to_classifier_class_dict={"tree":mlc.DecisionTreeClassifier, "svc":mlc.LinearSVC},
                       algorithm_name_to_classifier_model_class_dict={"tree":mlc.DecisionTreeClassificationModel, "svc":mlc.LinearSVC},
                       reload_preliminary_results=True,
                       absolute_path_prefix=os.path.abspath(os.path.join("", os.pardir)),
                       results_folder="Results",
                       models_folder="Models",
                       destination_folder="Results/Eval/Final",
                       selections_done_on_train_df=True,
                       flatten=False,
                       target_col="target",
                       eval_col="evaluation",
                       eval_prefixes=("val+test", "val", "test"),  # TODO: consider adding train as well
                       eval_sampling_techniques=("random", "EWU", "EU", "inter_EWU+EU", "tweet"),
                       eval_sampling_percentages=("1pct", "2pct", "5pct", "10pct"),
                       sorting_order=("trained_on", "algorithm", "note", "feature_selection"),
                       existing_evals_col="existing_evals_list",
                       missing_evals_col="missing_evals_list",
                       consider_all_evals=False,
                       initial_classification_done=True,
                       dev=False,
                       print_progress=True):

    prauc_evals = None
    rce_evals = None
    dev_prefix = "dev-" if dev else ""
    opposite_eval_prefix = "" if dev else "dev-"  # needed for <consider_all_evals>
    df_columns = ["algorithm", "note", "feature_selection", "trained_on", "evaluated_on"]
    df_columns_no_evaluated = ["algorithm", "note", "feature_selection", "trained_on"]
    assert algorithm_name_to_classifier_class_dict.keys() == algorithm_name_to_classifier_model_class_dict.keys()
    target_features = list(target_features)
    sorting_order = list(sorting_order)

    if os.path.exists(destination_folder) and os.path.isfile(
            os.path.join(destination_folder, dev_prefix + "final-prauc.csv")) \
            and os.path.isfile(os.path.join(destination_folder, dev_prefix + "final-rce.csv")):
        prauc_evals_original = pd.read_csv(os.path.join(destination_folder, dev_prefix + "final-prauc.csv"))
        rce_evals_original = pd.read_csv(os.path.join(destination_folder, dev_prefix + "final-rce.csv"))
        print("Cleaning and verifying prauc_evals_original and rce_evals_original.")
        prauc_evals_original, rce_evals_original = remove_duplicates_and_inconsistencies(prauc=prauc_evals_original, rce=rce_evals_original, key_columns=None, sorting_order=None, print_progress=print_progress)
        prauc_evals_original, rce_evals_original = flatten_deflatten_prauc_rce_as_needed(prauc_evals=prauc_evals_original, rce_evals=rce_evals_original, flatten=flatten, engs=target_features, target_col=target_col, eval_col=eval_col, print_progress=print_progress)
    else:
        if flatten:
            prauc_evals_original = pd.DataFrame(columns=df_columns + target_col + eval_col)
            rce_evals_original = pd.DataFrame(columns=df_columns + target_col + eval_col)
        else:
            prauc_evals_original = pd.DataFrame(columns=df_columns + target_features)
            rce_evals_original = pd.DataFrame(columns=df_columns + target_features)

    if reload_preliminary_results:
        for algorithm in algorithm_name_to_classifier_class_dict.keys():
            individual_evals_path = os.path.join(results_folder, "Eval", algorithm, "csv")
            if not os.path.exists(individual_evals_path):
                if print_progress:
                    print(individual_evals_path, "does not exist!")
                continue

            # read already existing preliminary evaluations
            eval_files = [f for f in os.listdir(individual_evals_path) if os.path.isfile(os.path.join(individual_evals_path, f))]
            # keep only those that do (not) begin with "dev-", if <dev>  is (not) True AND that were
            # hyperparameter-tuned
            eval_files = [os.path.join(individual_evals_path, f) for f in eval_files if (((f[:4] == "dev-") == dev) and ("-ht-" in f))]
            for file in eval_files:
                if print_progress:
                    print(f"Reading {file}")
                # https://prnt.sc/8vKFEpREa6yD
                df = pd.read_csv(file)
                # https://prnt.sc/-zjIeuI5Jekq
                df["trained_on"] = df.apply(lambda row: update_values(row["trained_on"], row["sample"], eval_prefixes),
                                            axis=1)
                df.rename(columns={"sample": "evaluated_on"}, inplace=True)
                df, _ = remove_duplicates_and_inconsistencies(prauc=df, rce=None, key_columns=None, sorting_order=None,
                                                              print_progress=False)
                df, _ = flatten_deflatten_prauc_rce_as_needed(prauc_evals=df, rce_evals=None, flatten=flatten,
                                                              engs=target_features, target_col=target_col,
                                                              eval_col=eval_col, print_progress=False)
                if "prauc" in file:
                    prauc_evals = pd.concat([prauc_evals, df], axis="index", ignore_index=True)
                elif "rce" in file:
                    rce_evals = pd.concat([rce_evals, df], axis="index", ignore_index=True)
                else:
                    raise ValueError("Unexpected name of the file, contains neither prauc nor rce:", file)

            if prauc_evals is None:
                prauc_evals = pd.DataFrame(columns=df_columns + target_col + eval_col) if flatten else pd.DataFrame(columns=df_columns + target_features)

            if rce_evals is None:
                rce_evals = pd.DataFrame(columns=df_columns + target_col + eval_col) if flatten else pd.DataFrame(columns=df_columns + target_features)

            prauc_evals = merge_and_drop_duplicates(prauc_evals_original, prauc_evals, sorting_order)
            rce_evals = merge_and_drop_duplicates(rce_evals_original, rce_evals, sorting_order)
            prauc_evals.to_csv(os.path.join(destination_folder, dev_prefix + "final-prauc.csv"), index=False)
            rce_evals.to_csv(os.path.join(destination_folder, dev_prefix + "final-rce.csv"), index=False)
    else:
        prauc_evals = prauc_evals_original
        rce_evals = rce_evals_original

    print("Cleaning and verifying merged prauc_evals and rce_evals.")
    prauc_evals, rce_evals = remove_duplicates_and_inconsistencies(prauc=prauc_evals, rce=rce_evals, key_columns=None, sorting_order=sorting_order, print_progress=print_progress)

    if consider_all_evals and os.path.exists(destination_folder) and os.path.isfile(
            os.path.join(destination_folder, opposite_eval_prefix + "final-prauc.csv")) \
            and os.path.isfile(os.path.join(destination_folder, opposite_eval_prefix + "final-rce.csv")):
        prauc_evals_opposite = pd.read_csv(os.path.join(destination_folder, opposite_eval_prefix + "final-prauc.csv"))
        rce_evals_opposite = pd.read_csv(os.path.join(destination_folder, opposite_eval_prefix + "final-rce.csv"))
        if dev:
              prauc_evals_opposite = get_only_1_and_2pct_subset_evals(prauc_evals_opposite)  # when dev == True, only 1% and 2% datasets are used for evaluation
              rce_evals_opposite = get_only_1_and_2pct_subset_evals(rce_evals_opposite)
        print("Cleaning and verifying prauc_evals_opposite and rce_evals_opposite.")
        prauc_evals_opposite, rce_evals_opposite = remove_duplicates_and_inconsistencies(prauc=prauc_evals_opposite, rce=rce_evals_opposite, key_columns=None, sorting_order=None, print_progress=print_progress)
        prauc_evals_opposite, rce_evals_opposite = flatten_deflatten_prauc_rce_as_needed(prauc_evals=prauc_evals_opposite, rce_evals=rce_evals_opposite, flatten=flatten, engs=target_features, target_col=target_col, eval_col=eval_col, print_progress=print_progress)
        reference_prauc_evals = merge_and_drop_duplicates(prauc_evals_opposite, prauc_evals, sorting_order)
        reference_rce_evals = merge_and_drop_duplicates(rce_evals_opposite, rce_evals, sorting_order)
        print("Cleaning and verifying reference_prauc_evals and reference_rce_evals.")
        reference_prauc_evals, reference_rce_evals = remove_duplicates_and_inconsistencies(prauc=reference_prauc_evals, rce=reference_rce_evals, key_columns=None, sorting_order=sorting_order, print_progress=print_progress)
    else:
        reference_prauc_evals = prauc_evals
        reference_rce_evals = rce_evals


    '''
    Look through the <algorithm><note><feature_selection><trained_on> columns of dfs and examine which evaluations are
    missing from <evaluated_on>. Then creates each missing combination from <eval_prefixes><eval_sampling_techniques>
    <eval_sampling_percentages>.
    '''
    group_by_cols = df_columns_no_evaluated + [target_col] if flatten else df_columns_no_evaluated
    # https://prnt.sc/tbUQckd5qKST
    existing_praucs = get_already_existing_evals(reference_prauc_evals, existing_evals_col=existing_evals_col,
                                                 group_by_cols=group_by_cols, evals_col="evaluated_on",
                                                 sorting_order=sorting_order)
    existing_rces = get_already_existing_evals(reference_rce_evals, existing_evals_col=existing_evals_col,
                                               group_by_cols=group_by_cols, evals_col="evaluated_on",
                                               sorting_order=sorting_order)

    # https://prnt.sc/S8wd_Y_I04fQ
    eval_targets_list = []
    for epercent in eval_sampling_percentages:
        if dev and (epercent != "1pct") and (epercent!= "2pc"):
            continue  # when dev == True, only 1% and 2% datasets are used for evaluation
        for etech in eval_sampling_techniques:
            for ep in eval_prefixes:
                eval_targets_list.append(ep + "_" + etech + "_sample_" + epercent)
    if not dev:
        eval_targets_list += eval_prefixes  # when dev == True, only 1% and 2% datasets are used for evaluation

    missing_praucs = get_missing_eval_targets(existing_praucs, eval_targets_list, missing_evals_col=missing_evals_col,
                                              existing_evals_col=existing_evals_col)
    missing_rces = get_missing_eval_targets(existing_rces, eval_targets_list, missing_evals_col=missing_evals_col,
                                            existing_evals_col=existing_evals_col)

    if missing_praucs.loc[missing_praucs[missing_evals_col] != missing_rces[missing_evals_col]].empty:
        if print_progress:
            print("PRAUC and  EVALS match, as expected.")
    elif missing_praucs.loc[missing_praucs[missing_evals_col] != missing_rces[missing_evals_col]].shape[0] == 1:
        if ((len(missing_praucs.loc[missing_praucs[missing_evals_col] != missing_rces[missing_evals_col]][missing_evals_col][0]) > 0)
                and (len(missing_rces.loc[missing_praucs[missing_evals_col] != missing_rces[missing_evals_col]][missing_evals_col][0]) == 0)):
            relevant_index = missing_praucs.index[missing_praucs[missing_evals_col] != missing_rces[missing_evals_col]].tolist()[0]
            missing_praucs.at[relevant_index, missing_evals_col] = missing_rces.at[relevant_index, missing_evals_col]
            missing_praucs.at[relevant_index, existing_evals_col] = missing_rces.at[relevant_index, existing_evals_col]
            print(f"Had to manually update the PRAUC table for index {relevant_index}: \n{missing_praucs.iloc[relevant_index]}")
        # https://prnt.sc/8Pr6ykEo5cwx ; https://prnt.sc/wWKSlVNoGT05 ; https://prnt.sc/GB_W4oOp2LtZ
        elif ((len(missing_praucs.loc[missing_praucs[missing_evals_col] != missing_rces[missing_evals_col]][missing_evals_col][0]) == 0)
              and (len(missing_rces.loc[missing_praucs[missing_evals_col] != missing_rces[missing_evals_col]][missing_evals_col][0]) > 0)):
            relevant_index = missing_rces.index[missing_praucs[missing_evals_col] != missing_rces[missing_evals_col]].tolist()[0]
            missing_rces.at[relevant_index, missing_evals_col] = missing_praucs.at[relevant_index, missing_evals_col]
            missing_rces.at[relevant_index, existing_evals_col] = missing_praucs.at[relevant_index, existing_evals_col]
            print(f"Had to manually update the RCE table for index {relevant_index}: \n{missing_rces.iloc[relevant_index]}")
        else:
            print("PRAUC and RCE evals mismatch with multiple rows mismatching! Returning prauc_evals, rce_evals, missing_rces, missing_praucs")
            return prauc_evals, rce_evals, missing_rces, missing_praucs
    else:
        print("PRAUC and RCE evals mismatch with multiple mismatches! Returning prauc_evals, rce_evals, missing_rces, missing_praucs")
        return prauc_evals, rce_evals, missing_rces, missing_praucs


    # remove rows where nothing is missing (https://prnt.sc/5iUMUQ5_i1b6):
    missing_evals = missing_praucs[missing_praucs[missing_evals_col].map(lambda l: len(l)) > 0]
    # Since we checked for mismatch above, we can only use one df from now on, so we don't need something like:
    # missing_rces = missing_rces[missing_rces[missing_evals_col].map(lambda l: len(l)) > 0]

    # convert to dict for an easier iteration (https://prnt.sc/yuGjc_Aegs5m):
    missing_evals = missing_evals.to_dict(orient="index")

    # load hypertuned parameters (https://prnt.sc/rCSizLGxMdix):
    relevant_algorithms_set = set()
    relevant_notes_set = set()
    for i in missing_evals:
        relevant_algorithms_set.add(missing_evals[i]["algorithm"])
        relevant_notes_set.add(missing_evals[i]["note"])

    best_params = {}
    for algorithm in relevant_algorithms_set:
        pickle_folder = os.path.join(absolute_path_prefix, "Results", "Eval", algorithm, "pkl")
        best_params[algorithm] = {}
        for note in relevant_notes_set:
            params_path = "params_for_classifier-" + algorithm + "-based_on-train-" + note  # always on train
            # e.g. dev-params_for_classifier-svc-based_on-itself-scaled, dev- added in <unpickle_file> function
            best_params[algorithm][note] = unpickle_file(name=params_path, path=pickle_folder,
                                                         print_confirmation=print_progress, dev=dev)

    # for new evaluations:
    models = {}
    new_prauc = {}
    new_rce = {}

    # evaluate and extract:
    for i in missing_evals:
        # https://prnt.sc/XQsFuTvRXURF
        next_batch_of_missing_evals = missing_evals[i][missing_evals_col]
        algorithm = missing_evals[i]["algorithm"]
        note = missing_evals[i]["note"]
        feature_selection = missing_evals[i]["feature_selection"]
        trained_on = missing_evals[i]["trained_on"]

        classifier_class = algorithm_name_to_classifier_class_dict[algorithm]
        classifier_model_class = algorithm_name_to_classifier_model_class_dict[algorithm]
        # We always use HP tuning based on the train dataset and fitting based on the target dataset.
        cved_on = trained_on.replace("val+test", "train").replace("val", "train").replace("test", "train")
        if cved_on in ('train', 'val', 'test', 'val+test',):
            cved_on = cved_on + "_random_sample_10pct"
        else:
            cved_on = cved_on.replace("2pct", "1pct").replace("5pct", "1pct")

        main_key = "=".join([algorithm, note, feature_selection, trained_on])
        models[main_key] = {}
        new_prauc[main_key] = {}
        new_rce[main_key] = {}
        features_note_model_name_additions = "" if note == "scaled" else "-" + note + "-"

        if print_progress:
            print(
                f"Now looking for models for {main_key}/{features_note_model_name_additions}, the following "
                f"{len(next_batch_of_missing_evals)} still missing: {next_batch_of_missing_evals}.")

        for target in target_features:
            if (not initial_classification_done) and (main_key not in models):
                continue  # the main_key was already removed from the dict for a previous target further down in code (https://prnt.sc/6oJOBTYOd4d0)

            # Path to load/save the model, e.g. classifier_model_of_type-svc-for_features-top_50-for_dataset-val_random_sample_1pct-based_on_dataset-val_random_sample_1pct-predicting_target-react-ht
            full_model_name = "classifier_model_of_type-" + algorithm + \
                              "-for_features-" + feature_selection + \
                              features_note_model_name_additions + \
                              "-for_dataset-" + trained_on + \
                              "-based_on_dataset-" + trained_on + \
                              "-predicting_target-" + target + "-ht"
            model_path = os.path.join(models_folder, algorithm, full_model_name)
            if(os.path.exists(model_path)):
                try:
                    models[main_key][target] = classifier_model_class.load(model_path)
                    model_read = True
                    if print_progress:
                        print(f"\tLoaded model {full_model_name} for {main_key}/{target}.")
                except (Py4JJavaError, IllegalArgumentException):
                    model_read = False
            else:
                model_read = False

            if not model_read:
                try:
                    # We always use HP tuning based on the train dataset and fitting based on the target dataset.
                    # So here we fetch the ht parameters (originally saved as: best_params[corresponding_cv_df][target][feature_selection] = {k.name:best_params_map[k] for k in best_params_map.keys()})
                    next_best_params = best_params[algorithm][note][cved_on][target][feature_selection]
                    if print_progress:
                        print(f"\t Model {full_model_name} could not be reloaded and has to be recreated! HT parameters found.")
                except (KeyError, TypeError) as error:
                    if initial_classification_done:
                        raise ValueError(f"Neither model {full_model_name} nor its HT parameters could not be reloaded!\n"
                                         f"Check why this is the case for algorithm={algorithm}; \nnote={note}; \ncved_on={cved_on}; \ntarget={target}; \nfeature_selection={feature_selection}. \n"
                                         f"Received error={error}.")
                    else:
                        print(f"\tWARNING: Neither model {full_model_name} nor its HT parameters could not be reloaded! "
                              f"Because initial_classification_done={initial_classification_done}, we skip this model "
                              f"evaluation. Revisit this when the initial classification is done. "
                              f"Until then, we removed {main_key} from the models/new_prauc/new_rce dicts.")
                        del models[main_key]
                        del new_prauc[main_key]
                        del new_rce[main_key]
                        continue

                tuned_classifier_instance = classifier_class(**next_best_params)
                ev_col = "ev__" + feature_selection + "__" + note + "__" + target
                ev_col = ev_col + "__sdotd" if selections_done_on_train_df else ev_col
                # https://prnt.sc/TOdaLLuG0ZOM / https://prnt.sc/l5tDY9HuB0BZ
                featuresColParam = tuned_classifier_instance.getParam("featuresCol")
                featuresColParamValue = tuned_classifier_instance.extractParamMap()[featuresColParam]
                if (featuresColParamValue == "selected_features") or (featuresColParamValue == ev_col.replace("__", "=")):
                    print(f"\tUpdated TCI's {full_model_name}'s FeaturesCol from '{featuresColParamValue}' to '{ev_col}'")
                    tuned_classifier_instance.set(featuresColParam, ev_col)

                models[main_key][target] = tuned_classifier_instance.fit(dfs[trained_on])
                models[main_key][target].write().overwrite().save(model_path)
                if print_progress:
                    print(
                        f"\tModel {full_model_name} for {main_key}/{target} could not be loaded! A new version was created and saved at {models_folder}.")

        if (not initial_classification_done) and (main_key not in models):
            continue  # the main_key was already removed from the dict for a previous target above (https://prnt.sc/6oJOBTYOd4d0)

        for next_eval in next_batch_of_missing_evals:
            if next_eval not in dfs:
                if dev and ("1pct" not in next_eval) and ("2pct" not in next_eval):
                    continue  # when dev == True, only 1% and 2% datasets are used for evaluation
                else:
                    raise ValueError(f"\t\t No {next_eval} in dfs: {dfs.keys()}!")

            print(f"\tStarting the next batch of evaluations! Next: {main_key} on {next_eval}.")
            new_prauc[main_key][next_eval] = {}
            new_rce[main_key][next_eval] = {}

            for target in target_features:
                if target not in models[main_key]:
                    raise ValueError(f"\t\t No {target} in models[{main_key}]: {models[main_key].keys()}!")

                ev_col = "ev__" + feature_selection + "__" + note + "__" + target
                ev_col = ev_col + "__sdotd" if selections_done_on_train_df else ev_col
                # https://prnt.sc/TOdaLLuG0ZOM / https://prnt.sc/l5tDY9HuB0BZ
                featuresColParam = models[main_key][target].getParam("featuresCol")
                featuresColParamValue = models[main_key][target].extractParamMap()[featuresColParam]
                if (featuresColParamValue == "selected_features") or (featuresColParamValue == ev_col.replace("__", "=")):
                    print(f"\t\tUpdated {full_model_name}'s FeaturesCol from '{featuresColParamValue}' to '{ev_col}'")
                    models[main_key][target].set(featuresColParam, ev_col)
                    models[main_key][target].write().overwrite().save(model_path)

                predictions = models[main_key][target].transform(dfs[next_eval])
                pred = [x[0] for x in predictions.select("prediction").collect()]
                gt = [x[0] for x in predictions.select(target).collect()]
                new_prauc[main_key][next_eval][target] = compute_prauc(pred, gt)
                new_rce[main_key][next_eval][target] = compute_rce(pred, gt)
                if print_progress:
                    print(f"\t\tEvaluation done for {target}: "
                          f"{new_prauc[main_key][next_eval][target]}/{new_rce[main_key][next_eval][target]} "
                          f"at {datetime.now().strftime('%d.%m.%Y %H:%M:%S')}.")

            # export the results
            try:
                prauc_evals = update_final_evals(old_evals=prauc_evals, new_evals_dict=new_prauc, main_key=main_key, evaluated_on=next_eval, flatten=flatten, target_col=target_col, eval_col=eval_col)
                rce_evals = update_final_evals(old_evals=rce_evals, new_evals_dict=new_rce, main_key=main_key, evaluated_on=next_eval, flatten=flatten, target_col=target_col, eval_col=eval_col)
                prauc_evals.to_csv(os.path.join(destination_folder, dev_prefix + "final-prauc.csv"), index=False)
                rce_evals.to_csv(os.path.join(destination_folder, dev_prefix + "final-rce.csv"), index=False)
                if print_progress:
                    print(f"___ Exported the eval for {main_key}/{next_eval} at "
                          f"{datetime.now().strftime('%d.%m.%Y %H:%M:%S')}. ___ ")
            except ValueError as e:
                print(f"WARNING, could not export {next_eval} (throwing away following results {new_prauc[main_key][next_eval], new_rce[main_key][next_eval]}: {e.__str__()}")
                del new_prauc[main_key][next_eval]
                del new_rce[main_key][next_eval]

    if not flatten:
        prauc_evals.set_index(["algorithm", "note", "feature_selection", "trained_on", "evaluated_on"],
                                  verify_integrity=True, inplace=True)
        rce_evals.set_index(["algorithm", "note", "feature_selection", "trained_on", "evaluated_on"],
                                verify_integrity=True, inplace=True)

    return prauc_evals, rce_evals, models, missing_praucs

\end{lstlisting}
