# Supplementary material for: Context-Based Tweet Engagement Prediction
Source: arXiv:2310.03147 source file (2023-09-28)
Supplement: Supplementary file 5 [file extractGraphRelations.tex]

\begin{lstlisting}[language=Python,showstringspaces=false,caption={The method used to extract follower and engagement relations of both the first and second degree}, label=lstExtractNewRelations]
from pyspark.sql.functions import lit


def extract_graph_relations(df, graph, acting_user="engaged_with_user_id", acted_upon_user="engaging_user_id",
                            graph_acting_column="following_id", graph_acted_upon_column="followed_id",
                            new_feature_name="graph_engagee_follows_engager_2d", graph_flag_column=None,
                            null_as_false=True, train_graph=None):
    """
    Extracts graph relations from graph and saved them as a new feature of df.

    Takes a graph (of the form <acting_user, acted_upon_user>) of some relations (e.g. follows, likes) and creates a 
    new column new_feature_name based on it that is added to the main df. Should train_graph be another 
    relation-graph (again of the form acting_user, acted_upon_user), the union of graph and train_graph will be used 
    inplace of graph. 
    """

    # make sure the name of id columns in graph and id are not the same, because this would corrupt the semi-left 
    # join at the end 
    if (acting_user == graph_acting_column) or (acted_upon_user == graph_acted_upon_column):
        raise ValueError("User ID column names for df and graph must be different!")

    if train_graph is not None:
        # if the same user pair is given in train and test/val graph, take the value from the latter
        train_graph = train_graph.join(graph, (train_graph[graph_acting_column] == graph[graph_acting_column]) & (
                    train_graph[graph_acted_upon_column] == graph[graph_acted_upon_column]), how="left_anti")
        graph = graph.union(train_graph).distinct()
        # check that there are no duplicates, due to the antijoin, this must never be the case
        if graph.count() != graph.distinct().count():
            raise ValueError("Unexpected result when merging train and test/val graph!")

    if graph_flag_column is None:
        if not isinstance(new_feature_name, str):
            raise ValueError("If gaph_flag_column is None, new_feature_name must be a string!")
        # if the graph has no indicator column, presume that all contained pairs are true
        graph = graph.withColumn(new_feature_name, lit(True))
        # in case there are other columns in the graph, disregard them
        graph = graph.select([graph_acting_column, graph_acted_upon_column, new_feature_name])

    elif isinstance(graph_flag_column, str) and isinstance(new_feature_name, str):
        graph = graph.withColumnRenamed(existing=graph_flag_column, new=new_feature_name)
        # in case there are other columns in the graph, disregard them
        graph = graph.select([graph_acting_column, graph_acted_upon_column, new_feature_name])

    elif isinstance(graph_flag_column, list) and isinstance(new_feature_name, list) and (len(graph_flag_column) == len(new_feature_name)):
        for existing, new in zip(graph_flag_column, new_feature_name):
            graph = graph.withColumnRenamed(existing=existing, new=new)

        # in case there are other columns in the graph, disregard them, notice the * before the list in new_feature_name
        graph = graph.select([graph_acting_column, graph_acted_upon_column, *new_feature_name])

    else:
        raise ValueError("Argument new_feature_name must not be None. If graph_flag_column is also not None, "
                         "then it must be either a string or a list and new_feature_name must be the same data type. "
                         "Moreover, if gaph_flag_column is a list, new_feature_name must have the same number of "
                         "elements.") 

    df = df.join(graph, (df[acting_user] == graph[graph_acting_column]) & (
                df[acted_upon_user] == graph[graph_acted_upon_column]),
                 how="left_outer").drop(graph_acting_column).drop(graph_acted_upon_column)

    if null_as_false:
        df = df.fillna(False, subset=new_feature_name)

    return df
\end{lstlisting}
