# Supplementary material for: Context-Based Tweet Engagement Prediction
Source: arXiv:2310.03147 source file (2023-09-28)
Supplement: Supplementary file 6 [file getCommonFactorCombinations.tex]

\begin{lstlisting}[language=Python,showstringspaces=false,caption={The method used to find the intersection of combinations of other factors for each value of the target factor}, label=lstGetCommonFactorCombinations]

def get_common_factor_combinations(main_df, factors_to_investigate=None, all_factors=None,
                                   exclude_prefixes=["eo_",], eval_cols=["evaluation",], target_col=None,
                                   look_at_all_together=True, return_found_counts=False, print_progress=True):
    """
    Groups the dataframe <main_df> by each column <f> in <factors_to_investigate> and then filters out all rows for the
    remaining columns in <all_factors> which do not appear in all <f> groups. Returns the filtered dfs in a dict with
    the <f> as the key. Example: https://prnt.sc/OjiVwq-h-Te-

    This function is equivalent to balance_dfs, but it is recommended when more than one factor is to be found.


    Parameters
    ----------
    main_df: dataframe to be filtered
    factors_to_investigate: a list of factors that will be the key columns
    all_factors: columns to be filtered
    exclude_prefixes: an interable with column prefixes which are to be excluded from factor investigation
    eval_cols: eval_cols to be carried over
    return_found_counts: whether to export a dataframe with exported details
    print_progress: whether to print how far along the calculation has progressed
    target_col: if there is a target column combining multiple evaluation types, this should specify that column
    look_at_all_together: whether to also try to find common combinations across all columns

    Returns
    -------
    the filtered df
    """

    if all_factors is None:
        # https://prnt.sc/sHzaCLyYejnC
        all_factors = [col for col in main_df.columns if col not in eval_cols]

    if factors_to_investigate is None:
        factors_to_investigate = all_factors

    if exclude_prefixes is not None:
        for ep in exclude_prefixes:
            all_factors = [col for col in all_factors if not col.startswith(ep)]
            factors_to_investigate = [col for col in factors_to_investigate if not col.startswith(ep)]

    if target_col is not None:
        engs = list(main_df[target_col].unique())

    results = {}
    special_string = "all factors combined"

    if look_at_all_together:
        factors_to_investigate.append(special_string)

    if return_found_counts:
        common_factors_dict = defaultdict(list)

    for f in factors_to_investigate:
        # https://prnt.sc/3funqbdgMxLn
        other_factors = [factor for factor in all_factors if (factor != f and factor != special_string)]
        # https://prnt.sc/sCpc1_ykjN0g
        df = main_df.copy(deep=True).dropna()
        # https://stackoverflow.com/a/33098470
        df["combi"] = df[other_factors].apply(lambda x: '-'.join(x.astype(str)), axis=1)
        if f != special_string:
            # https://prnt.sc/cIAou9tPh8kO
            f_combi_set = df.groupby(f)["combi"].agg(combi_set=set)
        else:
            f_combi_set = df["combi"].agg(combi_set=set)
        ## https://prnt.sc/nRgadN6QYduI
        #f_combi_intersection = reduce(lambda x, y: x.intersection(y), f_combi_set['combi_set'])
        # https://prnt.sc/cm8CC0QLlyMA ; https://prnt.sc/EgwvkVvFJWks
        f_combi_intersection = set.intersection(*f_combi_set['combi_set'])
        # https://prnt.sc/rZOQWltnnGKM
        df = df.loc[df["combi"].isin(f_combi_intersection)]
        # https://prnt.sc/1w1agC0BRbFL
        del df["combi"]
        if print_progress:
            if f != special_string:
                print(f"\tAt {datetime.now().strftime('%d.%m.%Y %H:%M:%S')} done with common factor {f} with values "
                      f"{df[f].unique()} and shape {df.shape}.")
            else:
                print(f"\tAt {datetime.now().strftime('%d.%m.%Y %H:%M:%S')} done with all factors together with shape "
                      f"{df.shape}.")
        if return_found_counts:
            common_factors_dict["factor"].append(f)
            common_factors_dict["calculated_dt"].append(datetime.now().strftime('%d.%m.%Y %H:%M:%S'))
            if f != special_string:
                common_factors_dict["values"].append(df[f].unique())
            else:
                common_factors_dict["values"].append(f)
            common_factors_dict["common_counts"].append(df.shape[0])
        if target_col is not None:
            results[f] = {}
            shapes = {}
            for eng in engs:
                results[f][eng] = df.loc[df[target_col] == eng]
                shapes[eng] = results[f][eng].shape
                if return_found_counts:
                    common_factors_dict[eng].append(shapes[eng][0])
            results[f]["all"] = df
            if print_progress:
                print(f"\t\t -> {shapes}.")
        else:
            results[f] = df
            common_factors_dict[target_col].append(df.shape[0])

    if return_found_counts:
        return results, pd.DataFrame(common_factors_dict)
    else:
        return results
\end{lstlisting}
