# Supplementary material for: Context-Based Tweet Engagement Prediction
Source: arXiv:2310.03147 source file (2023-09-28)
Supplement: Supplementary file 7 [file getFrequency.tex]

\begin{lstlisting}[language=Python,caption={The method that counts the appearances of indivdiaul tweet elements}, label=lstGetFrequency]
from pyspark.sql import functions as f
from pyspark.sql import Window
import sys

hours = lambda i: int(i * 3600)

def get_frequency(df, column_name="hashtags", group_by_cols=["item"], prior_hours=None, new_col_prefix="", new_col_suffix=""):
    """
    Counts the number of appearances of individual items (hashtags/links/domains), optionally for the given timeframe.

    df -- dataframe from which frequencies are extracted
    column_name -- target column name (expected "hashtags", "present_links", or "present_domains")
    group_by_cols -- set to ["item"] to get values for all tweets in the dataset; set it to ["engaging_user_id", "item"]
    to get values only for tweets seen by the user
    prior_hours -- None to consider the dataframe or the number of hours, cf. https://stackoverflow.com/a/33226511
    new_col_prefix -- e.g. the perspective, i.e. e.g. "viewed" or "total"
    new_col_suffix -- e.g. the time frame, i.e. e.g. 30min, 1h, etc.
    """

    new_col = resolve_column_naming(column_name, new_col_prefix, new_col_suffix)

    # split the list at \t https://prnt.sc/26i1er1
    start = df.select("tweet_id", "engaging_user_id", "tweet_timestamp", f.split(f.col(column_name), "\t").alias("help"))

    exploded = start.select("tweet_id", "engaging_user_id", "tweet_timestamp", f.explode(f.col("help")).alias("item"))

    if prior_hours is not None:
        w = (Window().partitionBy(*group_by_cols).orderBy(f.col("tweet_timestamp").cast("long")).
             rangeBetween(-hours(prior_hours), 0))
    else:
        w = (Window().partitionBy(*group_by_cols).orderBy(f.col("tweet_timestamp").cast("long")).
             rangeBetween(-sys.maxsize, 0))

    item_count = exploded.select(*group_by_cols, "tweet_timestamp", f.count("item").over(w).alias("count"))
    # old version without window:
    # item_count = f.exploded.groupBy(*group_by_f.cols).count()

    # without tweet_timestamp as a join condition, we'd have too many instances: 
    # compare https://prnt.sc/26ka723 ; https://prnt.sc/26ka9jd ; https://prnt.sc/26kaavm
    # with https://prnt.sc/26kabnh ; https://prnt.sc/26kai71
    joined = exploded.join(item_count, on=(group_by_cols+["tweet_timestamp"]))
    #joined = exploded.join(item_count, on=group_by_cols)
    # "tweet_id", "engaging_user_id" together identify an instance uniquely
    final = joined.groupBy("tweet_id", "engaging_user_id").agg(f.sum("count"))
    final = final.withColumnRenamed("sum(count)", new_col)
    df = df.join(final, on=["tweet_id", "engaging_user_id"], how="leftouter")

    return df


\end{lstlisting}
