# Supplementary material for: Context-Based Tweet Engagement Prediction
Source: arXiv:2310.03147 source file (2023-09-28)
Supplement: Supplementary file 8 [file predictAndEvaluate.tex]

\begin{lstlisting}[language=Python,caption={The method used to tune the hyperparameters and to fit and evaluate the initial classification models},label={lstPredictEvaluate}]
import pyspark.ml.classification as mlc  # for LogisticRegression, LogisticRegressionModel, etc.
from pyspark.ml.tuning import CrossValidator, ParamGridBuilder
from py4j.protocol import Py4JJavaError
from pyspark.sql.utils import AnalysisException

import os
from datetime import datetime
import pandas as pd
import numpy as np

from Functions.pp_calculate_evaluation_metrics import compute_prauc, compute_rce
from Functions.pp_get_already_existing_evals import get_already_existing_evals
from Functions.pp_update_preliminary_evals import update_preliminary_evals
from Functions.pp_mllib_rce_evaluator import RCEEvaluator
from Functions.pickle_file import pickle_file
from Functions.unpickle_file import unpickle_file
from Functions.pp_flatten_deflatten import flatten_deflatten_prauc_rce_as_needed
from Functions.pp_remove_duplicates_and_inconsistencies import remove_duplicates_and_inconsistencies
from Functions.pp_get_corresponding_train_key_and_prepare_best_params_dict import \
    get_corresponding_train_key_and_prepare_best_params_dict


def mllib_predict_evaluate(dfs,
                           target_features=('like', 'reply', 'retweet', 'quote', 'react',),
                           classifier_class=mlc.DecisionTreeClassifier,
                           classifier_model_class=mlc.DecisionTreeClassificationModel,
                           classifier_prefix="tree",
                           rewrite_existing_models=False,
                           force_model_reloading=False,
                           recreate_missing_models=True,
                           models_folder="Models",
                           csv_folder="Evals_csv",
                           pickle_folder="Eval_pkl",
                           features_note="scaled",
                           top_n_selected_list=["all", ],
                           flatten=False,
                           target_col="target",
                           eval_col="evaluation",
                           base_predictions_on_train_dfs=True,
                           selections_done_on_train_df=True,
                           hypertune_params=None,
                           layers=None,
                           dev=False,
                           print_progress=True):
    """
    This function loops for each dataframe in <dfs> and predicts targets from <target_features> based on explanatory
    features listed in <features_dict>. It uses the classifier from PySpark's mllib specified in <classifier_class>
    with the corresponding model's class specified in <classifier_model_class>.

    Parameters
    ----------
    dfs: a dictionary of dataframes with a vectorised column with explanatory features
    target_features: a list of target labels
    classifier_class: the class of the classifier from PySpark's mllib
    classifier_model_class: the class of the model of the classifier from PySpark's mllib
    classifier_prefix: the natural language name of the classifier
    models_folder: the name of the folder to save fitted classifier models in
    rewrite_existing_models: whether to recreate, refit, and rewrite classifier models
    force_model_reloading: whether to reload a model if its evaluation already exists
    recreate_missing_models: whether to recreate models which are missing, but whose evaluation already exists
    features_note: a note about features to be saved in evals (e.g. "scaled", "oracle", etc.)
    top_n_selected_list: list with top_n selected features to be considered (expected to be a subset of
        ['top_5', 'top_10', 'top_25', 'top_50', 'all'])
    csv_folder: the name of the folder to save/load evaluations in/from .csv format (if not None)
    pickle_folder: the name of the folder to save/load evaluations in/from .csv format (if not None)
    flatten: whether to only have one eval per row (if false, one row will contain evals for each of the target
        engagements); cf. https://prnt.sc/rG1HiIpkXTig and https://prnt.sc/Gk1sTMvAn-d3
    target_col: column name in the flattened form describing whose values are individual tweet engagement goals
    eval_col: column name in the flattened form describing with an individual evaluation value
    base_predictions_on_train_dfs: whether to fit on the corresponding train dataset instead of the same dataset
    selections_done_on_train_df: whether to fit on the features selected from the corresponding train dataset
    hypertune_params: the grid of hyperparameters to tune of form [(param1, value1), (param2, value2,),]
        or None if no tuning ought to be done
    layers: only relevant for hyperparameter tuning, contains a list of sets of layer sizes, with only the input layer
        empty. Is ignored if None.
    dev: whether dev mode is used; if True, "dev-" prefix will be used for CSV/pickle imports and exports
    print_progress: whether to print the fitting and prediction progress

    Returns
    -------
    fitted <models>, the sets <reloaded_models_set>, <rewritten_models_set>, and <skipped_models_set> as well as the
    updated evaluations <prauc_evals> and <rce_evals>
    """

    ### LOAD PREEXISTING EVALS ###
    based_on = "train" if base_predictions_on_train_dfs else "itself"
    hypertune_suffix = "-ht" if (hypertune_params is not None) else ""
    eval_path = "classifier-" + classifier_prefix + "-based_on-" + based_on + "-" + features_note + hypertune_suffix
    eval_path = "dev-" + eval_path if dev else eval_path
    params_path = "params_for_classifier-" + classifier_prefix + "-based_on-" + based_on + "-" + features_note
    if csv_folder is not None:
        eval_path = os.path.join(csv_folder, eval_path)

    if not rewrite_existing_models:
        try:
            prauc_evals = pd.read_csv(eval_path + "-prauc.csv")
            rce_evals = pd.read_csv(eval_path + "-rce.csv")
            prauc_evals, rce_evals = remove_duplicates_and_inconsistencies(prauc=prauc_evals, rce=rce_evals, key_columns=None, sorting_order=None, print_progress=print_progress)
            prauc_evals, rce_evals = flatten_deflatten_prauc_rce_as_needed(prauc_evals, rce_evals, flatten=flatten, engs=target_features, target_col=target_col, eval_col=eval_col, print_progress=print_progress)
            # also performs integrity confirmation
            already_existing_evals = get_already_existing_evals(prauc_evals=prauc_evals, rce_evals=rce_evals, flatten=flatten, recreate_missing_models=recreate_missing_models)
            if print_progress:
                print(f"From {eval_path}-prauc.csv and -rce.csv: \n Read prauc evals {prauc_evals.shape} and rce evals {rce_evals.shape}, of which non-NaN rows "
                      f"are {prauc_evals[~prauc_evals.isnull().any(axis=1)].shape}: {already_existing_evals}.")

        except FileNotFoundError:
            prauc_evals = {}
            rce_evals = {}
            already_existing_evals = set()
            if print_progress:
                print(f"{eval_path}-prauc.csv/-rce.csv do not exist.")
    else:
        prauc_evals = None
        rce_evals = None
        already_existing_evals = set()
        if print_progress:
            print(f"Recreating and reevaluating models for {classifier_prefix}")

    ### LOAD PREEXISTING MODELS ###
    models = {}
    reloaded_models_set = set()
    rewritten_models_set = set()
    skipped_models_set = set()
    # for new evaluations:
    new_prauc = {}
    new_rce = {}
    # for hyperparameter tuning:
    if (not rewrite_existing_models) and (pickle_folder is not None) and (hypertune_params is not None):
        best_params = unpickle_file(name=params_path, path=pickle_folder, print_confirmation=print_progress, dev=dev)
        if best_params is None:
            best_params = {}
    else:
        best_params = {}

    for sample in dfs:
        models[sample] = {}
        new_prauc[sample] = {}
        new_rce[sample] = {}
        corresponding_train_key = sample.replace("val+test", "train").replace("val", "train").replace("test", "train") \
            if base_predictions_on_train_dfs else sample

        for top_n_selected in top_n_selected_list:
            at_least_one_evaluation_done = False
            for target in target_features:
                ev_col = "ev__" + top_n_selected + "__" + features_note + "__" + target
                ev_col = ev_col+"__sdotd" if selections_done_on_train_df else ev_col
                if ev_col not in dfs[sample].columns:
                    if print_progress:
                        print(f"Skipping {ev_col} for {sample} because the column is missing.")
                    continue

                if target not in models[sample].keys():
                    models[sample][target] = {}
                    new_prauc[sample][target] = {}
                    new_rce[sample][target] = {}

                if flatten:
                    next_combo = (classifier_prefix, features_note, based_on, sample, top_n_selected, target,)
                    # e.g. ('bayes', 'scaled', 'itself', 'test_random_sample_1pct', 'all', 'like')
                else:
                    next_combo = (classifier_prefix, features_note, based_on, sample, top_n_selected,)
                    # e.g. ('bayes', 'scaled', 'itself', 'test_random_sample_1pct', 'all')

                ### PREDICT ###
                features_note_model_name_addition = "" if features_note == "scaled" else "-" + features_note + "-"
                full_model_name = "classifier_model_of_type-" + classifier_prefix + \
                                  "-for_features-" + top_n_selected + \
                                  features_note_model_name_addition + \
                                  "-for_dataset-" + sample + \
                                  "-based_on_dataset-" + corresponding_train_key + \
                                  "-predicting_target-" + target + \
                                  hypertune_suffix
                model_path = os.path.join(models_folder, full_model_name)

                # Attempt to load the model if allowed and it exists
                if rewrite_existing_models:
                    evaluate_model = True
                    create_model = True
                elif force_model_reloading or recreate_missing_models or (next_combo not in already_existing_evals):
                    try:
                        models[sample][target][top_n_selected] = classifier_model_class.load(model_path)
                        # In previous versions of the work that did not account for different feature notes,
                        # the ev_cal was always called "selected_features" or it used the restricted symbol "=" in
                        # column names, so we have to account for that here.
                        if (models[sample][target][top_n_selected].getFeaturesCol() == "selected_features") or \
                                (models[sample][target][top_n_selected].getFeaturesCol() == ev_col.replace("__", "=")):
                            models[sample][target][top_n_selected] = models[sample][target][top_n_selected].setFeaturesCol(ev_col)
                            models[sample][target][top_n_selected].write().overwrite().save(model_path)
                        reloaded_models_set.add(full_model_name)
                        evaluate_model = force_model_reloading

                        # check whether it is needed to save hyper-parameters again:
                        if (sample == corresponding_train_key) and (pickle_folder is not None) and (
                                hypertune_params is not None):
                            corresponding_cv_df, best_params = get_corresponding_train_key_and_prepare_best_params_dict(
                                best_params=best_params,
                                corresponding_train_key=corresponding_train_key,
                                target=target)
                            if top_n_selected not in best_params[corresponding_cv_df][target]:
                                best_params_map = models[sample][target][top_n_selected].extractParamMap()
                                best_params[corresponding_cv_df][target][top_n_selected] = {k.name: best_params_map[k]
                                                                                            for k in
                                                                                            best_params_map.keys()}
                                pickle_file(var=best_params, name=params_path, path=pickle_folder,
                                            print_confirmation=False, dev=dev)
                                if print_progress and force_model_reloading:
                                    print(f"\tLoaded {full_model_name} at {datetime.now().strftime('%d.%m.%Y %H:%M:%S')} for reevaluation. The hyperparameter were successfully reexported.")
                            else:  # hyperparameters for the model already exported
                                if print_progress and force_model_reloading:
                                    print(
                                        f"\tLoaded {full_model_name} at {datetime.now().strftime('%d.%m.%Y %H:%M:%S')} "
                                        f"for reevaluation. The hyperparameters had already existed and did not have "
                                        f"to be reexpoerted.")
                        else:  # no hyperparameters were tuned on this df sample
                            if print_progress and force_model_reloading:
                                print(f"\tLoaded {full_model_name} at {datetime.now().strftime('%d.%m.%Y %H:%M:%S')} "
                                      f"for reevaluation.")

                        create_model = False
                    except (Py4JJavaError, FileNotFoundError, AnalysisException) as error:
                        evaluate_model = True
                        create_model = True
                        if print_progress:
                            print(f"\tModel {full_model_name} does not exist, it will be recreated.")
                else:
                    evaluate_model = False
                    create_model = False
                    skipped_models_set.add(full_model_name)

                # Recreate the model if necessary
                if create_model:
                    if hypertune_params is None:
                        if layers is None:
                            classifier_instance = classifier_class(labelCol=target, featuresCol=ev_col)
                        else:
                            if type(layers[0]) != int:
                                layers = layers[0]
                            input_layer_size = len(dfs[sample].head()[ev_col])
                            layers = [input_layer_size] + layers
                            classifier_instance = classifier_class(labelCol=target, featuresCol=ev_col, layers=layers)
                        models[sample][target][top_n_selected] = classifier_instance.fit(dfs[corresponding_train_key])
                        models[sample][target][top_n_selected].write().overwrite().save(model_path)
                        rewritten_models_set.add(full_model_name)
                    else:  # do the hyperparameter tuning: https://spark.apache.org/docs/2.4.1/ml-tuning.html
                        corresponding_cv_df, best_params = get_corresponding_train_key_and_prepare_best_params_dict(
                            best_params=best_params,
                            corresponding_train_key=corresponding_train_key,
                            target=target)
                        if top_n_selected not in best_params[corresponding_cv_df][target]:
                            grid = ParamGridBuilder()
                            default_classifier_instance = classifier_class(labelCol=target, featuresCol=ev_col)
                            # <layers> only relevant if the classifier is a multilayer perceptron
                            if layers is not None:
                                input_layer_size = len(dfs[sample].head()[ev_col])
                                full_layers = [[input_layer_size] + list(other_layers) for other_layers in layers]
                                hypertune_params["layers"] = full_layers

                            for hp in hypertune_params:  # https://prnt.sc/YfXJjC59WeSO
                                grid = grid.addGrid(getattr(default_classifier_instance, hp), hypertune_params[hp])
                                # For a view of how this loop creates the hyperparameter grid, please cf.:
                                # https://stackoverflow.com/questions/3061/calling-a-function-of-a-module-by-using-its-name-a-string
                                # and https://spark.apache.org/docs/latest/api/python/reference/api/pyspark.ml.tuning.ParamGridBuilder.htm

                            grid = grid.build()
                            # https://stackoverflow.com/questions/51404344/custom-evaluator-in-pyspark
                            crossval = CrossValidator(estimator=default_classifier_instance,
                                                      estimatorParamMaps=grid,
                                                      evaluator=RCEEvaluator(predictionCol="prediction", labelCol=target),
                                                      numFolds=4,
                                                      seed=42)
                            # Run cross-validation, and choose the best set of parameters.
                            cv_model = crossval.fit(dfs[corresponding_cv_df])

                            # save the parameters into the dict:
                            # https://stackoverflow.com/questions/36697304/how-to-extract-model-hyper-parameters-from-spark-ml-in-pyspark
                            # https://prnt.sc/ekyr3-DU7WRZ ; https://prnt.sc/Pf66jKUYvunY ; https://prnt.sc/pn0eChJvBf1W
                            # ; https://prnt.sc/ppib34NKmD2a
                            best_params_map = cv_model.bestModel.extractParamMap()
                            best_params[corresponding_cv_df][target][top_n_selected] = {k.name: best_params_map[k] for k
                                                                                        in best_params_map.keys()}
                            # print("The best params ->", best_params[corresponding_cv_df][target][top_n_selected])
                            # return crossval, cv_model, best_params_map
                            pickle_file(var=best_params, name=params_path, path=pickle_folder,
                                        print_confirmation=print_progress, dev=dev)

                        tuned_classifier_instance = classifier_class(
                            **best_params[corresponding_cv_df][target][top_n_selected])
                        models[sample][target][top_n_selected] = tuned_classifier_instance.fit(
                            dfs[corresponding_train_key])
                        models[sample][target][top_n_selected].write().overwrite().save(model_path)
                        rewritten_models_set.add(full_model_name)

                    if print_progress:
                        print(f"\t\tTraining the model done at {datetime.now().strftime('%d.%m.%Y %H:%M:%S')}.")

                ### EVALUATE ###
                if evaluate_model:
                    at_least_one_evaluation_done = True
                    predictions = models[sample][target][top_n_selected].transform(dfs[sample])
                    pred = [x[0] for x in predictions.select("prediction").collect()]
                    gt = [x[0] for x in predictions.select(target).collect()]
                    new_prauc[sample][target][top_n_selected] = compute_prauc(pred, gt)
                    new_rce[sample][target][top_n_selected] = compute_rce(pred, gt)
                    if print_progress:
                        print(f"\t\t\tEvaluation done for {sample}/{target}: "
                              f"{new_prauc[sample][target][top_n_selected]}/{new_rce[sample][target][top_n_selected]} "
                              f"at {datetime.now().strftime('%d.%m.%Y %H:%M:%S')}.")

                    # export the results
                    prauc_evals = update_preliminary_evals(old_evals=prauc_evals, new_evals_dict=new_prauc, samples=[sample], classifier_prefix=classifier_prefix, based_on=based_on, features_note=features_note, flatten=flatten, target_col=target_col, eval_col=eval_col)
                    rce_evals = update_preliminary_evals(old_evals=rce_evals, new_evals_dict=new_rce, samples=[sample], classifier_prefix=classifier_prefix, based_on=based_on, features_note=features_note, flatten=flatten, target_col=target_col, eval_col=eval_col)
                    prauc_evals.to_csv(eval_path + "-prauc.csv", index=False)
                    rce_evals.to_csv(eval_path + "-rce.csv", index=False)
                    if print_progress:
                        print(f"\t\t\tExported the evaluation for to {eval_path}-prauc.csv "
                              f"and -rce.csv at {datetime.now().strftime('%d.%m.%Y %H:%M:%S')}.")

            if print_progress and at_least_one_evaluation_done:
                print(f"\t\t Done with all targets for {sample}/{top_n_selected} at "
                      f"{datetime.now().strftime('%d.%m.%Y %H:%M:%S')}.___")

        if print_progress:
            print(f"___ Done with all models for {sample} at {datetime.now().strftime('%d.%m.%Y %H:%M:%S')}. ___")

    if not flatten:
        prauc_evals.set_index(["algorithm", "note", "trained_on", "sample", "feature_selection"],
                              verify_integrity=True, inplace=True)
        rce_evals.set_index(["algorithm", "note", "trained_on", "sample", "feature_selection"],
                            verify_integrity=True, inplace=True)
    return models, reloaded_models_set, rewritten_models_set, skipped_models_set, prauc_evals, rce_evals

\end{lstlisting}
