# Supplementary material for: Context-Based Tweet Engagement Prediction
Source: arXiv:2310.03147 source file (2023-09-28)
Supplement: Supplementary file 10 [file vectoriseSelectedColumns.tex]

\begin{lstlisting}[language=Python,caption={This method vectorises columns with features to be used as input to classification algorithms}, label=lstVectorisation]
import pyspark.ml.feature as mlf
from Functions.export_dataframes import export_dataframes


def vectorise_selected_features(dfs,
                                changed_dfs,
                                selected_features_dict,
                                featureset_to_features_note_map={"relevant_features":"scaled",},
                                rewrite_existing_models=False,
                                export_prefix="ChiSq_",
                                export_dataforder="Data"):

    vec_dfs = {}

    for key in dfs:
        vec_dfs[key] = dfs[key]
        corresponding_train_key = key.replace("val+test", "train").replace("val", "train").replace("test", "train")

        for featureset in selected_features_dict[key]:
            note = featureset_to_features_note_map[featureset]
            for eng in selected_features_dict[key][featureset]:
                for top_n_selected in selected_features_dict[key][featureset][eng]:
                    # first we add the columns made on the dataset itself
                    ev_col = "ev__" + top_n_selected + "__" + note + "__" + eng
                    if rewrite_existing_models or (ev_col not in vec_dfs[key].columns):
                        if ev_col in vec_dfs[key].columns:
                            vec_dfs[key] = vec_dfs[key].drop(ev_col)  # https://spark.apache.org/docs/3.2.0/api/python/reference/api/pyspark.sql.DataFrame.drop.html
                        vec_assembler = mlf.VectorAssembler(inputCols=selected_features_dict[key][featureset][eng][top_n_selected],
                                                            outputCol=ev_col,
                                                            handleInvalid="error")
                        vec_dfs[key] = vec_assembler.transform(vec_dfs[key])
                        changed_dfs.add(key)
                        
                    
                    #then we add the columns made on the corresponding train dataset
                    ev_col_sdotd = ev_col + "__sdotd"  # selection done on train dataset
                    if rewrite_existing_models or (ev_col_sdotd not in vec_dfs[key].columns):
                        if ev_col_sdotd in vec_dfs[key].columns:
                            vec_dfs[key] = vec_dfs[key].drop(ev_col_sdotd)  # https://spark.apache.org/docs/3.2.0/api/python/reference/api/pyspark.sql.DataFrame.drop.html
                        vec_assembler = mlf.VectorAssembler(inputCols=selected_features_dict[corresponding_train_key][featureset][eng][top_n_selected],
                                                            outputCol=ev_col_sdotd,
                                                            handleInvalid="error")
                        vec_dfs[key] = vec_assembler.transform(vec_dfs[key])
                        changed_dfs.add(key)
                        
                    if key in changed_dfs:
                        export_dataframes(dfs={key:vec_dfs[key]}, featureset_export_prefix=export_prefix, 
                              HDFS_datafolder=export_dataforder, files_to_be_exported={key})
                        changed_dfs.remove(key)

    return vec_dfs, changed_dfs

\end{lstlisting}
