# Supplementary material for: Context-Based Tweet Engagement Prediction
Source: arXiv:2310.03147 source file (2023-09-28)
Supplement: Supplementary file 11 [file decodingText.tex]

\begin{lstlisting}[language=Python, caption={Code used to decode tweet text}, label=lstDecodeText]
from transformers import BertTokenizer, BertModel

tokenizer = BertTokenizer.from_pretrained('bert-base-multilingual-cased', do_lower_case=False)
model = BertModel.from_pretrained('bert-base-multilingual-cased')

def separate_and_decrypt(row):    
    if row is None:
        return ""
    
    tweet_tokens = row.split("\t")
    return "".join(tokenizer.convert_tokens_to_string(tokenizer.convert_ids_to_tokens(tweet_tokens)))

udf_separate_and_decrypt = f.udf(separate_and_decrypt, t.StringType())

for key in all_dfs:
    if (RECREATE_EVEN_IF_ALREADY_EXIST) or ("text" not in all_dfs[key].columns):
        all_dfs[key] = all_dfs[key].withColumn("text", udf_separate_and_decrypt(all_dfs[key]["text_tokens"]))
        print(f"Done with {key}.")
\end{lstlisting}
