# Supplementary material for: Context-Based Tweet Engagement Prediction
Source: arXiv:2310.03147 source file (2023-09-28)
Supplement: Supplementary file 12 [file last48h.tex]

\begin{lstlisting}[language=Python,caption={The code used to merge the last 48 hours of train subsets to the corresponding test, val, and test+val datasets}, label=lstLast48h]

from py4j.protocol import Py4JJavaError
from pyspark.sql.functions import col
from pyspark.sql.utils import AnalysisException

import os

from Functions.export_dataframes import export_dataframes


def help_import_appended_dataframes(spark, key, fix_different_ratio, hdfs_datafolder="Data", file_prefix="appended_"):
    """
    This function imports a single dataframe and returns it and a flag set to true if the dataset exists at the provided
    path. Otherwise, (None, False) is returned.
    """

    df = None
    file_loaded = False

    if fix_different_ratio:
        path = os.path.join(hdfs_datafolder, file_prefix + key + ".parquet")
    else:
        path = os.path.join(hdfs_datafolder, "full_" + file_prefix + key + ".parquet")

    try:
        df = spark.read.parquet(path)
        file_loaded = True
    except (Py4JJavaError, AnalysisException) as e:
        pass

    return df, file_loaded




def create_test_val_ds_with_days_from_train(spark, dfs:dict, changed_dfs:set, export_prefix:str,
                                            hdfs_datafolder:str,
                                            train_prefix="train", 
                                            other_prefixes=("val+test", "val", "test",), 
                                            calendar_days_to_be_copied=[42,43,],
                                            calendar_days_col="tweet_day_of_year", 
                                            fix_different_ratio=True,
                                            column_mismatch_okay=False):
    """
    Data Split

    For test and val we want to include the last days of train, as it precedes the beginning time of test and val.
    If the flag for fixing different ratio is set to true, then a random sample of the corrected ratio is added rather
    than all days (i.e. rather than 10 as many rows, due to the fact that train is 10 as big as train/val).
    """

    appended_dfs = {}
    
    for dfs_key in dfs:
        cmo = column_mismatch_okay or (dfs_key in changed_dfs)
        
        if train_prefix in dfs_key:
            appended_dfs[dfs_key] = dfs[dfs_key]
            continue

        other_found = False
        for other_prefix in other_prefixes:
            if (not other_found) and (other_prefix in dfs_key):
                other_found = True

                # return the dfs if already appended or create the appended dfs if it is not
                if dfs_key not in changed_dfs:
                    appended_dfs[dfs_key] = dfs[dfs_key]
                else:
                    train_key = dfs_key.replace(other_prefix, train_prefix)
                    last_train_days = dfs[train_key].filter(col(calendar_days_col).isin(calendar_days_to_be_copied))

                    # fix ratios (more instances in train than in test/val) datasets
                    if fix_different_ratio:
                        dfs_count = dfs[dfs_key].count()
                        train_count = dfs[train_key].count()
                        fraction = dfs_count/train_count
                        if fraction > 1:
                            print(f"Fixing ratios attempted, but not possible, because {dfs_key} has more instances ({dfs_count}) than {train_key} ({train_count})! Fraction={fraction}")
                        else:
                            print(f"Fixing ratios: {dfs_key} has {dfs_count} instances, {train_key} has {train_count} with fraction of {fraction}.")
                            last_train_days = last_train_days.sample(withReplacement=False, fraction=fraction, seed=42)

                    # append the two datasets
                    try:
                        appended_dfs[dfs_key] = last_train_days.unionByName(dfs[dfs_key])
                    except (AnalysisException, Py4JJavaError) as e:
                        if cmo:
                            common_cols = set(last_train_days.columns).intersection(set(dfs[dfs_key].columns))
                            appended_dfs[dfs_key] = last_train_days.select(*common_cols).unionByName(dfs[dfs_key].select(*common_cols))
                        else:
                            raise e
                    
                    # verify the datasets very appended correctly
                    if cmo:
                        assert (len(appended_dfs[dfs_key].columns) == len(dfs[dfs_key].columns)) or \
                               (len(appended_dfs[dfs_key].columns) == len(dfs[train_key].columns))
                    else:
                        assert len(last_train_days.columns) == len(dfs[dfs_key].columns)
                        assert len(appended_dfs[dfs_key].columns) == len(dfs[dfs_key].columns)
                    assert  (last_train_days.count() + dfs[dfs_key].count()) == appended_dfs[dfs_key].count()
                    
                    # export the appended dataframe
                    export_dataframes(dfs={dfs_key: appended_dfs[dfs_key]}, featureset_export_prefix=export_prefix,
                                      HDFS_datafolder=hdfs_datafolder)
                    # changed_dfs.add(dfs_key) not needed, since it was already exported
        
        # assert we did not have an unexpected prefix
        assert other_found

    return appended_dfs


\end{lstlisting}
